# Supplementary material for: Speeding up Learning Quantum States through Group Equivariant Convolutional Quantum Ans\"atze
Source: arXiv:2112.07611 source file (2023-09-14)
Supplement: Supplementary file 1 [file sm_heisenberg.pdf]

# Supplemental Material: Speeding up Learning Quantum States through Group Equivariant Convolutional Quantum Ansätze

Han Zheng,<sup>1,2,\*</sup> Zimu Li,<sup>2,†</sup> Junyu Liu<sup>\*,3,4,5,‡</sup> Sergii Strelchuk,<sup>2,§</sup> and Risi Kondor<sup>1,6,7,¶</sup>

<sup>1</sup>Department of Statistics, The University of Chicago, Chicago, IL 60637, USA

<sup>2</sup>DAMTP, Center for Mathematical Sciences, University of Cambridge, Cambridge CB30WA, UK

<sup>3</sup>Pritzker School of Molecular Engineering, The University of Chicago, Chicago, IL 60637, USA

<sup>4</sup>Chicago Quantum Exchange, Chicago, IL 60637, USA

<sup>5</sup>Kadanoff Center for Theoretical Physics, The University of Chicago, Chicago, IL 60637, USA

<sup>6</sup>Department of Computer Science, The University of Chicago, Chicago, IL 60637, USA

<sup>7</sup>Flatiron Institute, New York City, NY 10010, USA

(Dated: December 25, 2021)

∗: corresponding author.

In this Supplemental Material, we will provide more mathematical backgrounds and prove theorems given in the main text.

## CONTENTS

|                                                                 |   |
|-----------------------------------------------------------------|---|
| I. More facts about Schur-Weyl duality and $S_n$ representation | 1 |
| II. Equivalent between Young basis and $SU(d)$ -irrep basis     | 2 |
| III. Proofs of the density theorem                              | 2 |
| References                                                      | 6 |

## I. MORE FACTS ABOUT SCHUR-WEYL DUALITY AND $S_n$ REPRESENTATION

**Lemma I.1.** Any local part  $\hat{S}_i \cdot \hat{S}_j$  constituting a Heisenberg Hamiltonian  $H = \sum_{ij} J_{ij} \hat{S}_i \cdot \hat{S}_j$  can be written as

$$\hat{S}_i \cdot \hat{S}_j = \frac{1}{2}(ij) - \frac{1}{4}I.$$

*Proof.* Let us consider  $\hat{S}_1 \cdot \hat{S}_2$ . Expanded by definition,

$$\hat{S}_1 \cdot \hat{S}_2 = \frac{1}{2}(J_{12}^2 - J_1^2 - J_2^2),$$

where for now the subscripts on  $J^2$  denotes all sites  $J^2$  acting on. Under total spin basis, it is easy to see that

$$J_{12}^2 - J_1^2 - J_2^2 = \begin{pmatrix} 2 & 0 & 0 & 0 \\ 0 & 2 & 0 & 0 \\ 0 & 0 & 2 & 0 \\ 0 & 0 & 0 & 0 \end{pmatrix} - \frac{3}{4}I - \frac{3}{4}I = \begin{pmatrix} \frac{1}{2} & 0 & 0 & 0 \\ 0 & \frac{1}{2} & 0 & 0 \\ 0 & 0 & \frac{1}{2} & 0 \\ 0 & 0 & 0 & -\frac{3}{2} \end{pmatrix}.$$

While

$$(12) = \begin{pmatrix} 1 & 0 & 0 & 0 \\ 0 & 1 & 0 & 0 \\ 0 & 0 & 1 & 0 \\ 0 & 0 & 0 & -1 \end{pmatrix}.$$

∗ hanz98@uchicago.edu

† lizm@mail.sustech.edu.cn

‡ junyuliu@uchicago.edu

§ ss870@cam.ac.uk

¶ risi@cs.uchicago.edu

Therefore,

$$\hat{S}_1 \cdot \hat{S}_2 = \frac{1}{2}(J_{12}^2 - J_1^2 - J_2^2) = \frac{1}{2}((12) - \frac{1}{2}I).$$

This argument holds for any  $i, j$ , hence the proof follows.  $\square$

**Theorem I.2.** Let  $\langle \pi_{\text{SU}(d)} \rangle$  be the collection of all matrices on  $V^{\otimes n}$  generated by  $\pi_{\text{SU}(d)}$  (i.e., taking both linear spans and matrix products) and let  $\langle \pi_{S_n} \rangle$  be defined similarly. Note that  $\langle \pi_{S_n} \rangle$  is just the representation of  $\mathbb{C}[S_n]$ . Let  $M$  be an arbitrary matrix of  $V^{\otimes n}$ . If it commutes with  $\langle \pi_{\text{SU}(d)} \rangle$ , then  $M \in \langle \pi_{S_n} \rangle$ . If it commutes with  $\langle \pi_{S_n} \rangle$ , then  $M \in \langle \pi_{\text{SU}(d)} \rangle$ .

This theorem is proved by the so-called *double commutant theorem*, details can be found in [1].

**Theorem I.3** (Wedderburn Theorem). Given any  $S_n$ -irrep  $S^\lambda$ , let  $\text{End}(S^\lambda)$  denote the collection of linear transformation of  $S^\lambda$ . With respect to any basis, e.g., the Young basis,  $\text{End}(S^\lambda)$  is simply the collection of all  $\dim S^\lambda \times \dim S^\lambda$  matrices. As a vector space, the group algebra  $\mathbb{C}[S_n]$  is isomorphic with the direct sum of  $\text{End}(S^\lambda)$ :

$$\mathbb{C}[S_n] \cong \bigoplus_{\lambda \vdash n} \text{End}(S^\lambda).$$

We emphasize that being different from a  $\text{SU}(d) - S_n$  duality on  $V^{\otimes n}$ , each different  $\lambda$ , i.e., inequivalent  $S_n$ -irrep, appears only once in the above direct sum and the summation takes all kinds of Young diagrams  $\lambda$  of size  $n$ . In any case, restricting to each  $\lambda$ ,  $\pi_{\mathbb{C}[S_n]}$  produces all  $\dim S^\lambda \times \dim S^\lambda$  matrices and hence any matrix commuting with  $\pi_{\mathbb{C}[S_n]}$  should be a scalar.

## II. EQUIVALENT BETWEEN YOUNG BASIS AND $\text{SU}(d)$ -IRREP BASIS

**Lemma II.1.** Under  $\text{SU}(d) - S_n$  duality, sequential coupling Casimir operators commute with YJM-elements.

*Proof.* We prove the case for  $\text{SU}(2)$  for simplicity. For a fixed number  $k \leq n$  of coupled qubits,  $\text{SU}(2)$  has only one Casimir operator  $J_k^2 = (S_x^k)^2 + (S_y^k)^2 + (S_z^k)^2$ . General case for  $\text{SU}(d)$  follows immediately by considering all the  $d - 1$  Casimir operators constructed in [2] simultaneously.

As the Casimir operator,  $J_k^2$  commutes with  $\pi_{\text{SU}(2)}$ . Thus its matrix representation can be expanded by  $\mathbb{C}[S_k]$  by Theorem I.2. On the other hand, restricted to the first  $k$  qubits,  $J_k^2$  commutes with  $\pi_{\mathbb{C}[S_k]}$  because it is generated by  $(\pi_{\text{SU}(2)}, (\mathbb{C}^2)^{\otimes k})$ . Hence Wedderburn theorem forces  $J_k^2$  to be a scalar in different  $S_k$ -irreps. Matrices of this form are completely expressible by  $\text{GZ}_k \subset \text{GZ}_n$ . Therefore,  $J_k^2$  commutes with  $X_1, \dots, X_n$ .  $\square$

**Theorem II.2.** The YJM-elements are strictly diagonal under the  $\text{SU}(d)$  irrep basis. Conversely, sequentially coupled Casimir operators are strictly diagonal in the Young basis. Hence the  $\text{SU}(d)$  irrep basis and the Young basis are equivalent.

*Proof.* The proof has two steps, we first show that  $X_i$  is block-diagonal under  $\pi_{\text{SU}(d)}$ , then we verify that it is strict diagonal. We only discuss the  $\text{SU}(2)$ -case for brevity. Obviously, sequential coupling Casimir operators  $J_k^2$  are strictly diagonal under the total spin basis. They are restricted to scalars (spin labels) with respect to the decomposition  $(\mathbb{C}^2)^{\otimes n} = \bigoplus_{\lambda} W_{\lambda}^{\oplus m_{\text{SU}(2), \lambda}}$ . For any fixed YJM-element  $X_i$ , since different copies of  $W_{\lambda}$  must exhibit different eigenvalues (spin labels) under at least one  $J_k^2$  and since  $X_i$  commutes with all these  $J_k^2$ ,  $X_i$  should be block-diagonal with respect to each  $W_{\lambda}$ , no matter they are isomorphic or not.

Furthermore, since by Theorem I.2  $X_i$  commutes with the spin operator  $S_z^n$  whose eigenvalues (spin components) are nowhere identical within any  $\text{SU}(2)$ -irrep,  $X_i$  should be a scalar on each  $W_{\lambda}$ . That is,  $X_i$  is diagonal under the total spin basis which indicates it is also the Young basis [3, 4]. Note that the spin operator  $S_z^n$ , and hence the spin component can be used to distinguish basis states from different copies of any isomorphic  $S_n$ -irrep because they classify different permutation modules as explained in the main text. In the general  $\text{SU}(d)$  case,  $S_z^n$  is generalized to  $\frac{1}{2}d(d-1)$  operators to label these copied states [5]. By the same reason, these operators commute with  $X_i$ . Since each copied state is uniquely labeled by these operators, the second step for  $\text{SU}(d) - S_n$  duality follows.  $\square$

## III. PROOFS OF THE DENSITY THEOREM

**Lemma III.1.** Let  $E_{ij} \in \mathfrak{gl}(d, \mathbb{C})$  be the matrix unit with entry 1 at  $(i, j)$  and 0 elsewhere. Given any matrix  $A$ , let  $\mathcal{I} \subset \{1, \dots, d\} \times \{1, \dots, d\}$  be the index set of  $A$  assigned with nonzero off-diagonal entries  $c_{ij}$ . Then Lie subalgebra generated by  $\mathfrak{d}(d)$  and  $A$  contains

$$\mathfrak{d}(d) \bigoplus_{(i,j) \in \mathcal{I}} R_{ij},$$

where  $R_{ij}$  is the 1-dimensional root space spanned by  $E_{ij}$ .

*Proof.* For any diagonal matrix  $h = \text{diag}(h_1, \dots, h_d) \in \mathfrak{d}(d)$ , the Lie bracket  $[h, E_{kl}] = (h_k - h_l)E_{kl}$  gives the root  $a_{kl}(h) := h_k - h_l$  of  $E_{kl}$  under  $h$ . Let  $h := \sum_i \lambda_i E_{ii}$  with  $\lambda = (\lambda_i)$  being determined later. We define

$$M_1 := [h, A] = \left[ \sum_i \lambda_i E_{ii}, \sum_{k,l \in \mathcal{I}} c_{kl} E_{kl} \right] = \sum_{k,l \in \mathcal{I}} a_{kl}(E_{ii}) \lambda_i E_{kl} = \sum_{k,l \in \mathcal{I}} (a_{kl} \cdot \lambda) E_{kl}.$$

In the second step of the above computation, we omit all possible diagonal elements of  $A$ . This is legal because the Lie bracket of  $h$  with any diagonal part vanishes. Moreover, we set

$$M_2 := [h, [h, A]] = \sum_{k,l \in \mathcal{I}} (a_{kl} \cdot \lambda)^2 E_{kl}, \dots, M_{|\mathcal{I}|} := [h, \dots, [h, A] \dots] = \sum_{k,l \in \mathcal{I}} (a_{kl} \cdot \lambda)^{|\mathcal{I}|} E_{kl}.$$

Note that  $|\mathcal{I}|$  is the number of nonzero off-diagonal elements. Then let us consider the following *Vandermonde matrix*:

$$V(a_{kl} \cdot \lambda) = \begin{pmatrix} 1 & 1 & \dots & 1 \\ a_{k_1 l_1} \cdot \lambda & a_{k_2 l_2} \cdot \lambda & \dots & a_{k_{|\mathcal{I}|} l_{|\mathcal{I}|}} \cdot \lambda \\ \vdots & \vdots & \ddots & \vdots \\ (a_{k_1 l_1} \cdot \lambda)^{|\mathcal{I}|-1} & (a_{k_2 l_2} \cdot \lambda)^{|\mathcal{I}|-1} & \dots & (a_{k_{|\mathcal{I}|} l_{|\mathcal{I}|}} \cdot \lambda)^{|\mathcal{I}|-1} \end{pmatrix}.$$

Viewing  $\mathfrak{gl}(d, \mathbb{C})$  as a  $d \times d$ -dimensional vector space with  $E_{ij}$  as the standard basis, we note that  $V(a_{kl} \cdot \lambda)$  transforms vectors  $\{c_{kl} E_{kl}\}$  to  $\{M_r\}$ . If  $\det V(a_{kl} \cdot \lambda) = (-1)^{|\mathcal{I}|(|\mathcal{I}|-1)/2} \prod_{s < t} (a_{k_s l_s} \cdot \lambda - a_{k_t l_t} \cdot \lambda) \neq 0$ , then it has an inverse and the linear span of  $\{M_r\}$  just equals that of  $\{c_{kl} E_{kl}\}$  which turns out to be  $\bigoplus_{(i,j) \in \mathcal{I}} R_{ij}$  by definition. Basic theory from linear algebra tells us that the union of hyperplanes of finitely-many nonzero vectors, here are  $a_{k_s l_s} - a_{k_t l_t} \neq 0$  as roots, cannot cover the whole vector space. Thus we can always find some  $\lambda$  to fulfill the requirement.  $\square$

The crucial technique of using Vandermonde matrix is adapted from the classical paper [6] on generating semisimple Lie algebra. By Okounkov-Vershik approach [3], a root  $a_{kl}$  in our setting is obtained by all products of YJM-elements. The difference  $a_{k_s l_s} - a_{k_t l_t}$  is always nonzero for roots, but using high order products of YJM-elements leads to a practical problem for ansatz design. Fortunately, we can solve this problem in the setting of  $S_n$ -CQA ansatz as well as of QAOA. The solution is given after Theorem III.4.

**Definition III.2.** Given an arbitrary Hermitian matrix  $H_P$ , let  $\mathcal{G}_{H_P}$  be the underlying indices graph of  $H_P$ . The matrix  $H_P$  is *path-connected* if the associated graph  $\mathcal{G}_{H_P}$  is connected. For instance, the matrix

$$H_P = (E_{14} + E_{23} + E_{35} + E_{45}) + (E_{41} + E_{32} + E_{53} + E_{54})$$

is path-connected. However,

$$H'_P = (E_{14} + E_{23} + E_{55}) + (E_{41} + E_{32} + E_{55})$$

is disconnected. One can see by exchanging rows and columns that  $H'_P$  is block-diagonal. Path-connectedness is also seen in the famous Perron-Frobenius theorem which has lots of applications in graph theory.

**Lemma III.3.** Let  $H_P$  be a path-connected Hamiltonian. Then the generated Lie algebra  $\langle \mathfrak{d}(d), H_P \rangle = \mathfrak{gl}(d, \mathbb{C})$ . Especially, let us consider  $\mathfrak{d}_{\mathbb{R}}(d)$  consisting of all real-valued diagonal matrices. Generated over  $\mathbb{R}$ ,  $\langle i\mathfrak{d}_{\mathbb{R}}(d), iH_P \rangle_{\mathbb{R}} = \mathfrak{u}(d)$ .

*Proof.* By the previous lemma,

$$\mathfrak{d}(d) \bigoplus_{(i,j) \in \mathcal{I}} R_{ij} \subset \langle \mathfrak{d}(d), H \rangle.$$

Given any pair of indices  $i \neq j$ , since the underlying indices graph of  $H_P$  is path connected, we can always find a path  $i = i_0 \rightarrow i_1 \rightarrow \dots \rightarrow i_k \rightarrow i_{k+1} = j$  with no repeating indices for which  $(i_l, i_{l+1}) \in \mathcal{I}$ . Thus

$$E_{ij} = E_{i_0 i_{k+1}} = [\dots [[E_{i_0 i_1}, E_{i_1 i_2}], E_{i_2 i_3}], \dots, E_{i_k i_{k+1}}]$$

belongs to the generated Lie algebra. Since  $\mathfrak{gl}(d, \mathbb{C}) = \mathfrak{d}(d) \bigoplus_{(i,j)} R_{ij}$  for arbitrary  $i \neq j$ , we prove the first statement.

On the other hand, the real Lie algebra  $\langle i\mathfrak{d}_{\mathbb{R}}(d), iH_P \rangle_{\mathbb{R}}$  is definitely contained in  $\mathfrak{u}(d)$ . Since its complexification can be expanded as

$$\langle i\mathfrak{d}_{\mathbb{R}}(d), iH_P \rangle_{\mathbb{R}} + i\langle i\mathfrak{d}_{\mathbb{R}}(d), iH_P \rangle_{\mathbb{R}} = \langle \mathfrak{d}(d), H_P \rangle = \mathfrak{gl}(d, \mathbb{C})$$

and since any matrix from  $\mathfrak{gl}(d, \mathbb{C})$  is uniquely decomposed as the sum of a Hermitian and an skew-Hermitian matrices, we complete the proof.  $\square$

**Theorem III.4.** Let  $H_P$  be any path-connected Hamiltonian and let  $X_{GZ} \in \mathcal{GZ}_n$  denote a real linear combination of elements from  $\{X_i, X_i X_j, X_i X_j X_k, \dots\}$ . Given any  $S^\lambda$ , the subgroup  $H := \langle \exp(i\beta X_{GZ}), \exp(i\gamma H_P) \rangle$  is dense in  $U(\dim S^\lambda)$ . Thus the ansätze constructed by alternating exponentials can approximate any of eigenstate  $H_P$ .

*Proof.* Our aim is to show that  $\bar{H} = U(\dim S^\lambda)$ . Generally,  $H$  may not be a Lie group even it is a subgroup of  $U(\dim S^\lambda)$ . However, after taking closure,  $\bar{H}$  becomes a Lie subgroup of  $U(\dim S^\lambda)$  by Cartan's closed subgroup theorem. Then one can talk about the Lie algebra  $\mathfrak{h}$  of  $\bar{H}$ . By definition,  $\exp(i\beta X_{GZ}), \exp(i\gamma H_P) \in H \subset \bar{H}$ . Thus

$$iX_{GZ} = \left. \frac{d}{d\theta} \right|_{\theta=0} e^{i\theta X_{GZ}}, \quad iH_P = \left. \frac{d}{d\gamma} \right|_{\gamma=0} e^{i\gamma H_P} \in \mathfrak{h}.$$

Since  $\mathfrak{h}$  is a real Lie algebra, it is proper to generate it over  $\mathbb{R}$ . Thus Lemma III.3 tells us that  $\mathfrak{h}$  equals  $\mathfrak{u}(\dim S^\lambda)$ .

Even with the same Lie algebra, we cannot claim immediately that  $\bar{H} = U(\dim S^\lambda)$  because  $U(\dim S^\lambda)$  is not simply connected. Fortunately, some basic results from differential topology come to our rescue. By Cartan's closed subgroup theorem,  $\bar{H}$  is a closed embedded submanifold  $U(\dim S^\lambda)$ . Since  $\mathfrak{h} = \mathfrak{u}(\dim S^\lambda)$ ,  $\dim \bar{H} = \dim U(\dim S^\lambda)$ . Embedded submanifold with the same dimension of its ambient manifold should be open. Therefore,  $\bar{H}$  is both open and closed in the connected group  $U(\dim S^\lambda)$ . They must be identical.  $\square$

**Definition III.5.** For any standard Young tableau  $T$  of shape  $(\lambda_1, \dots, \lambda_k)$ , let  $Y_i := X_i + kI$ . The *shifted content vector*  $\beta_T$  measured by these elements only contains positive integers. Using shifted content vector facilitates the following proof. Measuring via second-order product  $Y_i Y_j$ , we obtain an  $(n \times n)$ -component vector  $\beta_T^{(2)}(r, s)$ . It can also be written as a real symmetric matrix  $(\beta_T)^T \beta_T$  and hence called *tensor product content vector*.

**Lemma III.6.** Different standard Young tableaux/Young basis elements have different tensor product content vector. Moreover, let  $T_i, T_j, T_k, T_l$  be four standard Young tableaux of size  $n$ . We require that  $T_i \neq T_j$  and  $T_k \neq T_l$ . If all underlying Young diagrams are the same, we further require that  $T_i \neq T_k$  or  $T_j \neq T_l$  (this requirement comes from the computation of roots above). Then

$$\beta_i^{(2)} - \beta_j^{(2)} \neq \beta_k^{(2)} - \beta_l^{(2)}$$

That is, when extended to tensor product content vectors, the differences of different standard Young tableaux are still different.

*Proof.* The first statement follows by the one-to-one correspondence between Young basis elements and content vectors [3, 4]. To prove the later one, we first look at differences of shifted content vectors

$$\beta_i - \beta_j, \quad \beta_k - \beta_l.$$

If they are different, then we finish the proof.

Suppose then  $\beta_i - \beta_j = \beta_k - \beta_l$ . Since  $\beta_k - \beta_l \neq 0$ ,

$$\beta_i - \beta_j = \beta_k - \beta_l \neq \beta_l - \beta_k.$$

Thus there must be some integer  $r \in \{1, \dots, n\}$  such that

$$\beta_i(r) - \beta_j(r) \neq \beta_l(r) - \beta_k(r) \Leftrightarrow \beta_i(r) + \beta_k(r) \neq \beta_j(r) + \beta_l(r).$$

If  $\beta_i(r) - \beta_k(r) = \beta_j(r) - \beta_l(r) \neq 0$ , then

$$\begin{aligned} \beta_i^{(2)}(r, r) - \beta_k^{(2)}(r, r) &= (\beta_i(r) - \beta_k(r))(\beta_i(r) + \beta_k(r)) \\ &\neq (\beta_j(r) - \beta_l(r))(\beta_j(r) + \beta_l(r)) = \beta_j^{(2)}(r) - \beta_l^{(2)}(r) \\ \Rightarrow \beta_i^{(2)}(r, r) - \beta_j^{(2)}(r, r) &\neq \beta_k^{(2)}(r, r) - \beta_l^{(2)}(r, r) \Rightarrow \beta_i^{(2)} - \beta_j^{(2)} \neq \beta_k^{(2)} - \beta_l^{(2)}. \end{aligned}$$

Suppose  $\beta_i(r) - \beta_k(r) = \beta_j(r) - \beta_l(r) = 0$  for all  $r$  such that  $\beta_i(r) + \beta_k(r) \neq \beta_j(r) + \beta_l(r)$ , i.e.,  $\beta_i(r) = \beta_k(r)$  and  $\beta_j(r) = \beta_l(r)$ . Since  $\beta_i - \beta_j = \beta_k - \beta_l \neq 0$ ,

$$\beta_i(r) - \beta_j(r) = \beta_k(r) - \beta_l(r) \neq 0, \text{ i.e., } \beta_i(r) \neq \beta_j(r), \beta_k(r) \neq \beta_l(r).$$

Since  $T_i \neq T_k$  (otherwise,  $T_j$  must be different from  $T_l$  and that finishes the proof), there must be some  $s$  such that  $\beta_i(s) \neq \beta_k(s)$ . Again since  $\beta_i - \beta_j = \beta_k - \beta_l$ ,  $\beta_j(s) \neq \beta_l(s)$ . Since shifted content vectors only take positive integers as their components,

$$\begin{aligned} \beta_i(r)\beta_i(s) - \beta_k(r)\beta_k(s) &= \beta_i(r)(\beta_i(s) - \beta_k(s)) \neq 0 \\ &\neq \beta_j(r)(\beta_i(s) - \beta_k(s)) = \beta_j(r)(\beta_j(s) - \beta_l(s)) = \beta_j(r)\beta_j(s) - \beta_l(r)\beta_l(s) \\ \implies \beta_i^{(2)}(r, s) - \beta_j^{(2)}(r, s) &= \beta_i(r)\beta_i(s) - \beta_j(r)\beta_j(s) \\ &\neq \beta_k(r)\beta_k(s) - \beta_l(r)\beta_l(s) = \beta_k^{(2)}(r, s) - \beta_l^{(2)}(r, s). \end{aligned}$$

This finishes the proof.  $\square$

Combining Lemma III.6 with Lemma III.1,  $\langle iY_k Y_l, H_P \rangle$  can generate all the off-diagonal root spaces  $R_{ij}$  if  $H_P$  is path-connected. To complement the missing diagonal elements ( $iY_k Y_l$  is not enough to generate whole  $\text{GZ}_n$ ), we note that  $[E_{ij}, E_{ji}] = E_{ii} - E_{jj}$ . Thus all traceless diagonal matrices can be generated from  $\langle iY_k Y_l, H_P \rangle$ . Since, for instance,  $X_2$  is diagonal with a nonzero trace, all diagonal matrices can be generated. In conclusion, we obtain the following theorem.

**Theorem III.7.** *The subgroup generated by  $Y_k Y_l$  with a path-connected Hamiltonian  $H_P$  is still dense. Since  $Y_k Y_l = (X_k + kI)(X_l + kI) = X_k X_l + k(X_k + X_l) + k^2 I$  and since  $\exp(i\theta I)$  is simply a phase term, a  $S_n$ -CQA ansatz is written as*

$$\cdots \exp(-i \sum_{k,l} \beta_{kl} X_k X_l) \exp(-i\gamma H_P) \exp(-i \sum_{k,l} \beta'_{kl} X_k X_l) \exp(-i\gamma' H_P) \cdots,$$

where we redefine  $X_1$  as  $I$  with which any first-order YJM-element  $X_i$  can be written as  $X_i X_1$ .

To prove the universality of QAOA and reuse the above method on Pauli  $Z$  matrices and computational basis  $\{|e_i\rangle\}$ , we need to redefine Cartan subalgebra and roots. It is well-known that all diagonal Pauli basis elements  $\tilde{Z}_{r_1 \dots r_s} := Z_{r_1} \otimes \cdots \otimes Z_{r_s}$  are able to span any diagonal matrix under  $\{|e_i\rangle\}$  which in turn forms the Cartan subalgebra of  $\mathfrak{gl}(\mathbb{C}, 2^n)$ . We denote by  $\beta_i(j)$  the eigenvalue of  $|e_i\rangle$  measured by  $Z_j$ . Let  $E_{kl}$  be the matrix unit as in Lemma III.1 but under  $\{|e_i\rangle\}$ . The root  $a_{kl}$  of  $E_{kl}$  is given by

$$a_{kl}(j)E_{kl} = \text{ad}_{Z_j}(E_{kl}) = (\beta_k(j) - \beta_l(j))E_{kl}.$$

High order components of  $a_{kl}$  under  $\tilde{Z}_{r_1 \dots r_s}$  are obtained by products. With all these substitutions, Lemma III.1, Lemma III.3 and Theorem III.4 follow straightforward. We now examine that a local Hamiltonian  $H_Z = \sum \beta_{kl} Z_k Z_l$  consisting of first- and second-order product of Pauli  $Z$  ( $Z_0 = I$ ) also guarantees the universality. With the same spirit of Lemma III.6, we have

**Lemma III.8.** *Let  $v$  be any computational basis element. Then for any  $u_1 \neq v_1, u_2 \neq v_2$  (if  $u_1 = u_2$ , we require  $v_1 \neq v_2$  and vice versa),*

$$\beta_{u_1}^{(2)} - \beta_{v_1}^{(2)} \neq \beta_{u_2}^{(2)} - \beta_{v_2}^{(2)}.$$

*Proof.* One can take this lemma as a corollary of Lemma III.6 where content vectors are replaced by eigenvalues of  $Z_j$ . Since they only take values from  $\{\pm 1\}$ , there is a more straightforward way towards the proof by induction. Suppose the statement is true for  $n-1$  qubits. Let  $u_1, v_1, u_2, v_2$  be distinct computational basis elements from the  $n$ -qubit system. Possible assignments of their spins of the last qubit are listed in the following:

$$\begin{array}{cccc} (0, 0, & 0, 0), & (0, 0, & 1, 1), & (1, 1, & 0, 0), & (1, 1, & 1, 1), \\ (0, 1, & 0, 1), & (1, 0, & 1, 0), & (0, 1, & 1, 0), & (1, 0, & 0, 1), \\ (0, 0, & 0, 1), & (0, 0, & 1, 0), & (0, 1, & 0, 0), & (1, 0, & 0, 0), \\ (0, 1, & 1, 1), & (1, 0, & 1, 1), & (1, 1, & 0, 1), & (1, 1, & 1, 0). \end{array}$$

The last ten cases can be confirmed immediately as differences of eigenvalues measured by  $Z_n$  on the last qubit are different. We need to analyze the cases like  $(0, 0, \dots, 1, 1)$ . Deleting the last qubits, suppose then  $u_1 = u_2$  and  $v_1 = v_2$ . Since we require  $u_1 \neq v_1, u_2 \neq v_2$ , there exists some  $i < n$  such that  $\beta_{u_1}(i) - \beta_{v_1}(i) = \beta_{u_2}(i) - \beta_{v_2}(i) \neq 0$ . Then their eigenvalues of  $Z_i Z_n$  will provide the difference. If  $u_1 \neq u_2$  or  $v_1 \neq v_2$ , then by induction, we obtain the proof.  $\square$

Finally we have:

**Theorem III.9.** *Let  $H_X$  be the uniform summation of Pauli  $X$  operators or any other path-connected Hamiltonian on computational basis, the QAOA-ansatz generated by  $H_X, H_Z = \sum \beta_{kl} Z_k Z_l$  is dense in  $\text{U}(2^n)$ , i.e., it is universal.*

- 
- [1] R. Goodman and N. R. Wallach, *Symmetry, Representations, and Invariants* (Springer New York, 2009).
  - [2] L. C. Biedenharn, *Journal of Mathematical Physics* **4**, 436 (1963).
  - [3] A. Okounkov and A. Vershik, *Selecta Mathematica* **2**, 581 (1996).
  - [4] T. Ceccherini-Silberstein, F. Scarabotti, and F. Tolli, *Representation Theory of the Symmetric Groups* (Cambridge University Press, 2009).
  - [5] G. E. Baird and L. C. Biedenharn, *Journal of Mathematical Physics* **4**, 1449 (1963).
  - [6] M. Kuranishi, *Nagoya Mathematical Journal* **2**, 63 (1951).
